# Supplementary material for: DeepMesh: Differentiable Iso-Surface Extraction
Source: arXiv:2106.11795 source file (2022-03-24)
Supplement: Supplementary file 1 [file svr_shapenet_supp.tex]

\begin{table*}[h]
    \caption{\textbf{Single view reconstruction results on ShapeNet Core.} \BG{Do we wanna keep this?} Exploiting end-to-end differentiability to perform image-based refinement allows us to outperform all prior methods also in terms of F-Score.}
    %Metrics are CD ($\times 0.001$, the smaller the better), EMD ($\times 100$, the smaller the better), IoU (\%, the larger the better) and F-score (\%, the larger the better).}
	\label{tab:shapenet_supp}
	\begin{center}
		\scalebox{0.65}{
			\begin{tabular}{c|c|ccccccccccccc|c}
				\Xhline{2\arrayrulewidth}
				Metric & Method & plane & bench & cabinet & car & chair & display & lamp & speaker & rifle & sofa & table & phone & boat & mean \\
				\Xhline{2\arrayrulewidth}
				\multirow{6}{*}{F-Score$\%$ $\uparrow$}&AtlasNet &91 & 86 &74 &94 &91 &84 &81 &80 &96 &91 &91 &90 &90 & 89 \\
                &Pixel2Mesh&88 & 95 & \textbf{94} & 97 & 94 & 92 & 89 & 89 & 95 & \textbf{96} & 93 & 97 & 94 & 93 \\
                &Mesh R-CNN& 87&91 &90 &95 & 90 & 89 & 83 & 85 & 93 & 92 & 90 & 95 & 91 & 90 \\
                &DISN&94&94&89&96&90&92&78&85&96&\textbf{96}&87&96&93&91 \\
				\cline{2-16}
				&DeepMesh(raw)&92&95&92&98&94&91&85&86&96&94&91&95&93&91\\
				&DeepMesh&\textbf{96}&\textbf{97}&\textbf{94}&\textbf{98}&\textbf{97}&\textbf{95}&\textbf{91}&\textbf{91}&\textbf{98}&\textbf{96}&\textbf{94}&\textbf{98}&\textbf{95}&\textbf{95}\\
				\Xhline{2\arrayrulewidth}
		\end{tabular}}
	\end{center}
\end{table*}
